# Supplementary material for: Who Is the Strongest Enemy? Towards Optimal and Efficient Evasion Attacks in Deep RL
Source: arXiv:2106.05087 source file (2023-03-20)
Supplement: Supplementary file 1 [file fig_visualize.tex]

%!TEX root = ../0_iclr2021_evasionrl_main.tex

\vspace*{-0.5em}
\begin{figure}[!htbp]
\centering
	\begin{subfigure}[t]{0.49\columnwidth}
		\centering
		\includegraphics[width=0.8\textwidth]{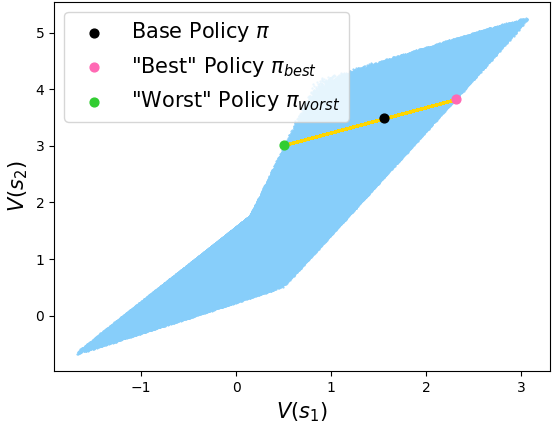}
	\caption{}
	\label{sfig:bracket}
	\end{subfigure}
	\hfill
	\begin{subfigure}[t]{0.49\columnwidth}
		\centering
		\includegraphics[width=0.8\textwidth]{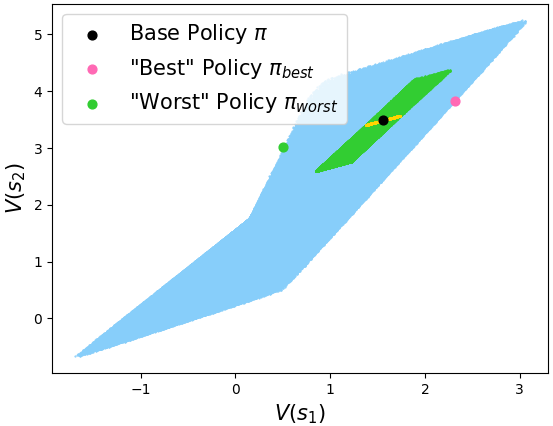}
	\caption{}
	\label{sfig:perturb}
	\end{subfigure}
	\vspace*{-1em}
	\caption{\small{\textbf{(a)} The values of all policies in $\Pi$ form a polytope (blue region); the values of all policies agreeing on all but one state $s$ form a line segment (yellow line), bracketed by two policies that are deterministic at $s$. \textbf{(b)} Perturb a given $\pi$ to $\tilde{\pi}$ within a connected and compact subset of policies $\ball(\pi) \subseteq \Pi$, the values of perturbed policies also form a polytope (green region), or a line segment if only perturb $\pi$ on one state. }}
	\label{fig:visualize}
\end{figure}
\vspace*{-0.5em}
